# Supplementary material for: SyncViolinist: Music-Oriented Violin Motion Generation Based on Bowing and Fingering
Source: arXiv:2412.08343 source file (2024-12-11)
Supplement: Supplementary file 1 [file ex1.tex]

To meet the needs of our model training task, we post-processed the recorded audio, motion, and bowing/fingering information.

First, to extract audio features from the recorded signals, we used librosa, a Python library for music signal processing ~\cite{Mcfee:15}. We applied a short-time Fourier transform (STFT) with a sliding window of length 2048 samples and a hop size of 1/30 seconds to obtain a 128-dimensional Mel-scaled spectrogram $X\in \mathbb{R}^{T \times 128}$. 

Next, we used Shogun\footnote{\url{https://www.vicon.com/software/shogun/}}, a motion editing software, to process the motion data and obtain the rotation information in Euler angles for 61 joints and the 3D positions of the root (24 for the body and 38 for the fingers). Next, we downsampled the motion data to 30 fps and calculated the 3D joint position $Y\in \mathbb{R}^{T \times 62 \times 3}$ from the rotation representation using forward kinematics, where $T$ represents the number of time frames. Additionally, we retargeted the motion data to a common skeleton to eliminate the effect of variations in the violinists' body sizes and shapes while keeping their hand and fingertip positions intact. 

Finally, to obtain the fingering and bowing information that is synchronized with the motion data, we used both the recorded MIDI signals and the MusicXML scores that were annotated by the violinists. It is worth noting that the MIDI signals were recorded simultaneously with the audio signals; thus, by annotating each label of the bowing/fingering information for each MIDI note, synchronization of audio features and bowing/fingering information can also be guaranteed at the same time. Since the bow direction and finger number labels were annotated in MusicXML by the violinists themselves, we were able to correspond the bow direction and finger number labels for each MIDI note actually played by synchronizing the MusicXML with the MIDI signals using a MIDI-to-score alignment method~\cite{Nakamura:17}.    
However, since this alignment is sometimes inaccurate, we manually corrected the information. 
For string labels, we obtained them by identifying which of the four channels had the largest output at each time frame since the MIDI violin used in our dataset acquisition process had outputs from different channels for each of the four strings.
As for position labels, we decided them from the recorded MIDI note number (\textit{i.e.}, pitch), played string, and the finger number obtained above.

After annotating each label in bowing/fingering information to the MIDI notes, we converted them to ensure that they were consistent with the time frame of audio features.
