# Supplementary material for: SyncViolinist: Music-Oriented Violin Motion Generation Based on Bowing and Fingering
Source: arXiv:2412.08343 source file (2024-12-11)
Supplement: Supplementary file 2 [file ex1.5.tex]

To ensure the diversity of the dataset, we conducted a comprehensive analysis covering both motion patterns and the music pieces included. Figure~\ref{fig:motion_stat} presents statistics on the key motion components of the dataset, while Fig.~\ref{fig:wrist_stat} illustrates the variation in the right wrist's speed. Additionally, Figs.~\ref{fig:bpm_stat}, \ref{fig:key_stat}, and \ref{fig:pitch_stat} demonstrate the diversity of the musical pieces included in the proposed dataset.
