# Supplementary material for: SyncViolinist: Music-Oriented Violin Motion Generation Based on Bowing and Fingering
Source: arXiv:2412.08343 source file (2024-12-11)
Supplement: Supplementary file 3 [file ex2.tex]

Figure~\ref{fig:subject_eval} presents the detailed results of the subjective evaluation. The left side shows the naturalness evaluation compared to other state-of-the-art methods, while the right side shows the naturalness evaluation compared to other ablative conditions.
Tracks 1 and 2, 3 to 5, and 6 to 8 correspond to the test data of players 1, 2, and 3, respectively.
