# Supplementary material for: SyncViolinist: Music-Oriented Violin Motion Generation Based on Bowing and Fingering
Source: arXiv:2412.08343 source file (2024-12-11)
Supplement: Supplementary file 4 [file ex3.tex]

Diagrams of the captured joints are illustrated in Fig.~\ref{fig:joints}. Furthermore, additional lists (Tables~\ref{table:joint_list1} and~\ref{table:joint_list2}) give the details of the joints available in the proposed dataset.
To benchmark the dataset, we re-implemented previous models with minimal modifications (i.e. only reshaping
the input and output dimensions, see Table~\ref{table:reshape_stat}) to account for the different numbers of key points.
